# Supplementary material for: Private Information Acquisition and Preemption: a Strategic Wald Problem
Source: arXiv:2207.02898 source file (2022-07-06)
Supplement: Supplementary file 1 [file put_to_appendix.tex]

In well-behaved problems, the value function $\hat{V}^{i}$ is a classical solution to the HJB equation (\ref{eq:hjbequation}).
In our problem, (\ref{eq:hjbequation}) may not be well-behaved as
$
\mathbb{E}_{t}\left[u_{\omega}^{R}\right]
$
may not be continuous everywhere given player $j$'s strategy and as
$
U^{i}\left(t\right)
$
may have discontinuities and kinks.
In the following discussion, I first show how player $j$'s strategy determines player $i$'s expected action-$R$ payoff.
Then, I show why this expected payoff may not be continuous everywhere and how its (dis)continuity affects player $i$'s best response.

Player $j$'s strategy induces conditional distributions over the time at which she takes an action.
These distributions then induce a distribution over player $i$'s action-$R$ payoff at each time $t$.
I first show how a player's strategy induces the conditional distributions over the time at which she takes an action.
Let
$
F_{\omega}^{j}\left(t\right)
$
be the probability that player $j$ takes action $R$ before or at time $t$ in state $\omega$.
Let
$
G_{\omega}^{j}\left(t\right)
$
be the probability that player $j$ takes action $S$ before or at time $t$ in state $\omega$.
Then,
$
1-
F_{\omega}^{j}\left(t\right)
-
G_{\omega}^{j}\left(t\right)
\geq
0
$
is the probability that player $j$ continues acquiring information at time $t$ in state $\omega$.
Here are some examples of the strategies and their induced distributions.

\begin{example}[Pure stopping]
\label{eg:purestrategy}
\normalfont
Consider player $j$'s pure strategy $(T^{j}, R)$.
This induces 
$
F_{\omega}^{j}\left(\cdot\right)
$
and 
$
G_{\omega}^{j}\left(\cdot\right)
$
as follows:
\begin{align*}
F_{H}^{j}\left(t\right)
=
\begin{cases}
1-e^{-at} 
& \text{if } t<T^{j}\\
1 
& \text{if } t\geq T^{j}
\end{cases}    
,
\text{ }
&
G_{H}^{j}\left(t\right)
=
0  
\end{align*}
and
\begin{align*}
F_{L}^{j}\left(t\right)
=
\begin{cases}
0 
& \text{if }t<T^{j}\\
e^{-bT^{j}} 
& \text{if }t\geq T^{j}
\end{cases}    
,
\text{ }
&
G_{L}^{j}\left(t\right)
=
\begin{cases}
1-e^{-bt} 
& \text{if } t<T^{j}\\
1- e^{-bT^{j}} 
& \text{if } t\geq T^{j}
\end{cases}  
.
\end{align*}

When player $j$ uses a pure strategy, 
the randomness of the stopping time comes from the randomness of the Poisson signal. 
In state $H$,
$
F_{H}^{j}\left(t\right),
$
the probability of player $j$ taking action $R$ before time $t<T^{j}$, 
is the probability of the arrival of the Poisson signal.
In the event of no revealing signal, player $j$ takes action $R$ at time $T^{j}$.
There is hence a positive probability that player $j$ takes action $R$ at time $T^{j}$.
This probability mass equals the probability of no revealing signal before time $T^{j}$.
In state $L$, 
$
F_{L}^{j}\left(t\right),
$
the probability of player $j$ taking action $R$ before time $t<T^{j}$ is zero. 
This is because in the event that player $j$ receives the revealing signal, player $j$ takes action $S$, and in the event of no revealing signal, player $j$ is still acquiring the signal.
In absence of the signal, player $j$ takes action $R$ at time $T^{j}$.
As a result, there is a positive probability that player $j$ takes action $R$ at time $T^{j}$ and this probability mass equals the probability of no revealing signal before time $T^{j}$.
\end{example}

\begin{example}[Randomised stopping]
\label{eg:randomisedstoppingtimemixedstrategy}
\normalfont
Consider player $j$'s mixed strategy when  $\sigma^{j}=0$.
If $\rho^{j}(t)$ is differentiable everywhere, 
then player $j$ takes action $R$ at each time $t$ with rate 
$
\frac{\frac{d\rho^{j}\left(t\right)}{dt}}{1-\rho^{j}\left(t\right)}
$.
She only takes action $S$ after receiving the $L$-state revealing signal.
This mixed strategy induces 
$
F_{\omega}^{j}\left(\cdot\right)
$
and 
$
G_{\omega}^{j}\left(\cdot\right)
$
as follows:
\begin{align*}
F_{H}^{j}\left(t\right) 
& 
=
\intop_{0}^{t}\left[e^{-as}\left(1-\rho^{j}\left(s\right)\right)\left(a+\frac{\frac{d\rho^{j}\left(s\right)}{ds}}{1-\rho^{j}\left(s\right)}\right)\right]ds
\\
& 
=
1-e^{-at}\left(1-\rho^{j}\left(t\right)\right),
\\
G_{H}^{j}\left(t\right)
&=0 
\end{align*}
and
\begin{align*}
F_{L}^{j}\left(t\right) 
&
=\intop_{0}^{t}\left[e^{-bs}\left(1-\rho^{j}\left(s\right)\right)\frac{\frac{d\rho^{j}\left(s\right)}{ds}}{1-\rho^{j}\left(s\right)}\right]ds
\\
&
=\intop_{0}^{t}\left[e^{-bs}\frac{d\rho^{j}\left(s\right)}{ds}\right]ds
,
\\
G_{L}^{j}\left(t\right)
&=
\intop_{0}^{t}\left[e^{-bs}\left(1-\rho^{j}\left(s\right)\right)b\right]ds
\end{align*}

In state $H$, player $j$ stops and takes action $R$ at time $t$ either because she receives an $H$-state revealing signal or because of her strategy $\rho^{j}$.
Conditional on arriving at time $t$, she stops and takes action $R$ at time $t$ with a rate 
$
a+\frac{\frac{d\rho^{j}\left(t\right)}{dt}}{1-\rho^{j}\left(t\right)}
$.
In state $L$, player $j$ stops and takes action $R$ at time $t$ if her strategy $\rho^{j}$ prescribes it. 
Conditional on arriving at time $t$, she stops and takes action $R$ at time $t$ with a rate 
$
\frac{\frac{d\rho^{j}\left(t\right)}{dt}}{1-\rho^{j}\left(t\right)}.
$
\end{example}

Next, 
I discuss the continuity of 
$
\mathbb{E}_{t}\left[u_{\omega}^{R}\right]
$
and 
$
U^{i}\left(t\right).
$
The main observation is that the continuity of 
$
U^{i}\left(t\right)
$
and
$
\mathbb{E}_{t}\left[u_{\omega}^{R}\right]
$
depends on that of 
$
F_{\omega}^{j}\left(t\right).
$
%When player $j$ uses a pure strategy (as in \Cref{eg:purestrategy}), the expected payoff
%$
%\mathbb{E}_{t}\left[u_{\omega}^{R}\right]
%$
%has a discontinuity point at $T^{j}$.
When player $j$ uses a mixed strategy (as in \Cref{eg:randomisedstoppingtimemixedstrategy}), both
$
\mathbb{E}_{t}\left[u_{\omega}^{R}\right]
$
and
$
U^{i}\left(t\right)
$
are continuous everywhere.
This is because the induced
$F_{\omega}^{j}\left(\cdot\right)$ is continuous everywhere and 
$\lim_{t\rightarrow0}F_{\omega}^{j}\left(t\right)=0$ for $\omega \in \{H,L\}$.
Then at each time $t$,
the distribution over player $i$'s payoff $u_{\omega}^{R}$ is a two-point distribution where 
\begin{align}
\label{eq:distributionofpayoffwhennojump}
u_{\omega}^{R}
=
\begin{cases}
u_{\omega}
&
\text{w.p. }1-F_{\omega}^{j}\left(t\right)
\\
u_{\omega}-\bar{\triangle}_{\omega}
&
\text{w.p. }F_{\omega}^{j}\left(t\right)
\end{cases}
.
\end{align}
Since $F_{\omega}^{j}\left(\cdot\right)$ is continuous, 
$
\mathbb{E}_{t}\left[u_{\omega}^{R}\right]
$
is also continuous.
%The expected payoff
%$
%\mathbb{E}_{t}\left[u_{\omega}^{R}\right]
%$
%may be upper semicontinuous at time $0$.
%If $F_{\omega}^{j}\left(\cdot\right)$ is continuous everywhere with $\lim_{t\rightarrow0}F_{\omega}^{j}\left(t\right) \neq 0$,
%then at time $t>0$, the distribution over player $i$'s payoff $u_{\omega}^{R}$ is as in (\ref{eq:distributionofpayoffwhennojump}), 
%but at time $0$, it is
%\begin{align*}
%u_{\omega}^{R}
%=\begin{cases}
%u_{\omega}
%&
%\text{w.p. }1-F_{\omega}^{j}\left(0\right)
%\\
%u_{\omega}-\underline{\triangle}_{\omega}
%&
%\text{w.p. }F_{\omega}^{j}\left(0\right)
%\end{cases}
%.
%\end{align*}
%The
%$
%\mathbb{E}_{t}\left[u_{\omega}^{R}\right]
%$
%function is then upper semicontinuous at $t=0$ and continuous everywhere else.
%This upper semicontinuity comes from the fact that player $j$ takes action $R$ with a positive mass at time $0$. 
%At time $t=\epsilon>0$, if player $i$ brings forward action $R$ by $\epsilon$, she gets the higher simultaneous-move payoff rather than second-mover payoff.
When 
$
\mathbb{E}_{t}\left[u_{H}^{R}\right]
$
is continuous, function $U^{i}\left(t\right)$ inherits its continuity from 
$
\mathbb{E}_{t}\left[u_{H}^{R}\right]
$ 
but can still have a kink because of the safe action payoff.
For a given player $j$'s strategy, player $i$'s value function is a viscosity solution to the HJB equation (\ref{eq:hjbequation}).
Qualitatively, player $i$'s best response has the following features.
When prior is extreme, player $i$'s best response is to take an immediate action $R$ or $S$ that achieves $U^{i}\left(0\right)$. 
When prior is in the intermediary range, player $i$ acquires information at time $0$.
As belief drifts up, player $i$ continues to acquire information when the marginal gain is greater than the marginal cost.
When the marginal gain and marginal cost are the same, player $i$ is indifferent between continuing and stopping and she randomises.
As discussed in \Cref{subsec:singleDM}, in the single DM case, the marginal gain depends only on the belief itself and does not depend on time $t$ directly. 
The smooth pasting condition pins down a (unique) cutoff belief at which the DM is indifferent between stopping and continuing. 
This is different from the single DM case. 
When player $j$ uses a mixed strategy,
player $i$'s marginal gain depends both on the belief 
$p_{t}$
and the current time
$t$
\footnote{
This is because player $j$'s mixed strategy can depend on $t$.}.
Given some of player $j$'s mixed strategies, the marginal gain and marginal cost can be the same not just for a time instant, but for a period of time.
She stops randomly with a positive rate when she is indifferent between stopping and continuing.

When player $j$ uses a pure strategy as in \Cref{eg:purestrategy},
the expected payoff 
$
\mathbb{E}_{t}\left[u_{\omega}^{R}\right]
$
has a discontinuity point at $T^{j}$.
If $F_{\omega}^{j}\left(\cdot\right)$ is discontinuous at some $T^{j}>0$ with $\lim_{t\rightarrow0}F_{\omega}^{j}\left(t\right) = 0$, 
then at time $t \neq T^{j}$, the distribution over player $i$'s action $R$ payoff is as in (\ref{eq:distributionofpayoffwhennojump}).
But at time $T^{j}$ the distribution over player $i$'s action $R$ payoff $u_{\omega}^{R}$ is
\begin{align*}
u_{\omega}^{R}
=
\begin{cases}
u_{\omega}
&
\text{w.p. }1-F_{\omega}^{j}\left(T^{j}\right)
\\
u_{\omega}-\underline{\triangle}_{\omega}
&
\text{w.p. }F_{\omega}^{j}\left(T^{j}\right)-F_{\omega}^{j}\left(T^{j}\right)_{-}
\\
u_{\omega}-\bar{\triangle}_{\omega} 
&
\text{w.p. }F_{\omega}^{j}\left(T^{j}\right)_{-}
\end{cases}
\footnotemark
.
\end{align*}
\footnotetext{
Let $f:\mathbb{R}\rightarrow \mathbb{R}$ be a function.
Let $f\left(c\right)_{-}$ denote the limit of $f\left(x\right)$ when $x$ approaches $c$ from the left, 
and let $f\left(c\right)_{+}$ denote the limit of $f\left(x\right)$ when $x$ approaches $c$ from the right.}
This is because player $j$ takes action $R$ with a positive mass of 
$
F_{\omega}^{j}\left(T^{j}\right)-F_{\omega}^{j}\left(T^{j}\right)_{-}
$  
at time $T^{j}$. 
Intuitively,
$
\mathbb{E}_{t}\left[u_{\omega}^{R}\right]
$
has a downward jump at $t=T^{j}$ such that 
$$
\lim_{t\rightarrow T^{j}_{-}}\mathbb{E}_{t}\left[u_{\omega}^{R}\right]
>
\mathbb{E}_{T^{j}}\left[u_{\omega}^{R}\right]
>
\lim_{t\rightarrow T^{j}_{+}}\mathbb{E}_{t}\left[u_{\omega}^{R}\right].
$$
%The $U^{i}\left(t\right)$ function inherits its (dis)continuity from 
%$\mathbb{E}_{t}\left[u_{\omega}^{R}\right]$.
%When $U^{i}\left(t\right)$ is neither lower nor upper semicontinuous at some bounded $T^{j}<\infty$, player $i$'s best response is to preempt.
%Suppose player $j$ uses the pure strategy 
%$
%(T^{j},R).
%$
%This strategy will induce discontinuous 
%$
%U^{i}\left(t\right)
%$
%at $t=T^{j}$.
%Consider the situation that player $i$ is at time infinitesimal close to $T^{j}$, denoted $T^{j}-dt$.
%Suppose if she stops at $T^{j}-dt$, it is optimal to take action $R$.
%Given the discontinuous 
%$
%U^{i}\left(t\right)
%$ 
%at 
%$
%t=T^{j},
%$
%the marginal gain from acquiring information at time $T^{j}-dt$ for $dt$ longer is negative.
%This is because first, the marginal change of belief in a short time $dt$ is negligible. 
%Second, in the event that player $j$ has not received the revealing signal before time $T^{j}-dt$, according to the strategy, player $j$ will stop at time $T^{j}$ and take action $R$ for certain.
%In this event, if player $i$ stops at time $T^{j}-dt$ and takes action $R$, she will get the first action $R$ taker payoff.
%However, 
%if player $i$ acquires the signal for $dt$ longer and take action $R$ at time $T^{j}$, then, she will only get the simultaneous-move payoff, which is strictly lower compared to taking action $R$ at time $T^{j}-dt$.
%The marginal gain from acquiring the signal for $dt$ longer at time $T^{j}-dt$ is hence negative.
%As a result, if player $i$ arrives at time $T^{j}-dt$, then, she has an incentive to preempt player $j$ and stop immediately.
This downward jump gives player $i$ the incentive to stop acquiring information at the time that is infinitesimal close to $T^{j}$ but slightly earlier.
This preemption motive can lead to unravelling.
